# Supplementary material for: Exhaustive Search of Ligand Binding Pathways via Volume-based Metadynamics
Source: arXiv:1904.10726 ancillary file (2019-04-24)
Supplement: Supplementary file 1 [file SI.pdf]

# Exhaustive Search of Ligand Binding Pathways via volume-based Metadynamics

## Supplementary Information

### Supplementary Note 1: Entropic correction

The translational entropy $S$ of a molecule of mass $m$ at temperature $T$ is given by[1]

$$S = R \log \left( \pi^{3/2} e^{5/2} \frac{V}{N} \lambda^3 \right) \tag{1}$$

where $R$ is the gas constant, and $\lambda = h/\sqrt{2mkT}$ is the De Broglie wavelength. We want to compute the difference between the translational entropy of the standard condition ($S^0$), and the entropy of the confined molecule inside the sphere ($S_\mathrm{s}$). The contribution given to the free energy by this difference can be computed using explicitly the equation (1)

$$\begin{aligned} T\Delta S &= T(S^0 - S_\mathrm{s}) \\ &= RT \log \left( \pi^{3/2} e^{5/2} \frac{1}{C^0} \lambda^3 \right) - RT \log \left( \pi^{3/2} e^{5/2} (V_\mathrm{s} - V_\mathrm{prot}) \lambda^3 \right) \\ &= RT \log \left( \frac{V^0}{\frac{4}{3}\pi\rho_\mathrm{s}^3 - V_\mathrm{prot}} \right) \end{aligned} \tag{2}$$

where $C^0$ is the standard concentration of 1/1660 Å$^{-3}$, $V_\mathrm{s}$=$\frac{4}{3}\pi\rho_\mathrm{s}^3$ is the volume of the restraining potential, and $V_\mathrm{prot}$ is the volume of the protein inside the sphere.
We thus obtain the final expression of the corrected $\Delta G_b^0$

$$\Delta G_b^0 = -RT \log \left( C^0 K_b \right) = \Delta G_\mathrm{MetaD} - RT \log \left( \frac{V^0}{\frac{4}{3}\pi\rho_\mathrm{s}^3 - V_\mathrm{prot}} \right) \tag{3}$$

### Supplementary Note 2: Details on the MD and system preparation

The initial protein structure was obtained from the X-ray structure of T4L /benzene complex (PDB code: 1L84[2]). It was immersed in ~10,000 water molecules. 8 $Cl^-$ ions were added to neutralize the system. We used the Amber14SB[3] force

field for protein and counterions, and TIP3P[4] for water. For the ligand we used the generalized AMBER force field (GAFF).[5] The atomic charges were obtained by the restrained electric potential fitting method (RESP)[6] with molecular electric potentials obtained in the HF/6-31G* level of theory. Quantum chemical calculations were performed with Gaussian 09.[7] Periodic boundary conditions were applied. Constant temperature simulations were achieved using the velocity rescaling thermostat[8] with solvent and solute coupled to separate heat baths with coupling constants of 0.5 ps. The pressure was maintained constant using an isotropic variant of the Parrinello-Rahman barostat[9,10] with a reference pressure of 1 bar, a coupling constant of 1 ps, and a compressibility of $4.5 \cdot 10^{-5}$ bar$^{-1}$. The time-step was 2 fs. Long range electrostatics interactions were computed with PME method[11] using a grid spacing of 1 Å.

The system energy was minimized by performing 2,000 steps of steepest descent algorithm, followed by 2,000 steps of conjugate gradient. With heavy atoms of protein and ligand fixed, the system was we heated up to 300 K for 2 ns in the NVT ensemble, followed by a 5 ns NPT simulation at 1 bar, 10 ns equilibration run without any constrains.

From the last equilibrated conformation, we performed 200 ns-long WT-MetaD runs biasing our three CVs (that we recall are the spherical coordinates $\rho, \theta, \varphi$). In particular, we performed one run for different values of $\rho_s$, namely 20,22,24,26, and 28 Å, with an confinement harmonic constant $k$=10 kJ/mol/Å$^2$, for a total of five production runs. A hill with a height of 1.2 kJ/mol was deposited every ps, the bias factor $\gamma$ was set to 20, sigmas for $\rho, \theta$, and $\varphi$ were set to 1 Å, $\frac{\pi}{16}$ rad, and $\frac{\pi}{8}$ rad respectively. The system is realigned every step to maintain the reference frame and the CVs fixed. We move the system' coordinates to align the position of the C-terminal domain to its equilibrated conformation (red in Figure 1 in main text).

## Supplementary Note 3: Description of the binding pathways

- **A**: The benzene ligand passes between helices D and E and exit to the solvent between helices C and F.

- **B**: the benzene ligand follows the initial direction of pathway **A**, but exiting between helices C and D

- **C**: The benzene ligand moves toward the helices H, I, and J and exits interacting with helices F,G and H.

- **D**: The benzene ligand moves toward the turn between helices E and D, and reaches the solvent interacting with helices H and J (near the turn between helices H and G and the end of helix J).

- **E**: The benzene ligand passes between helices G and D.

- **F**: The benzene ligand follows the same initial path of **C**, but when it exits does not interact with helices G and H, but with I and F.
- **G**: The benzene ligand passes in between the helices H, I and J.
- **H**: The benzene ligand enters through helices E and J (only binding direction, see Figure 4 in main text).

## PLUMED input file for $\rho_s$ = 20 Å

```
WHOLEMOLECULES ENTITY0=1-2593 ENTITY1=2594-2605
FIT_TO_TEMPLATE REFERENCE=heavy_atoms.pdb TYPE=OPTIMAL

sph: GROUP NDX_FILE=index.ndx NDX_GROUP=sphere
bnz: GROUP NDX_FILE=index.ndx NDX_GROUP=BNZ_noH
WRAPAROUND ATOMS=bnz AROUND=sph

sph_center: COM ATOMS=sph
bnz_center: COM ATOMS=bnz

sph_coord: POSITION ATOM=sph_center NOPBC
bnz_coord: POSITION ATOM=bnz_center NOPBC
abs_x: MATHEVAL ARG=bnz_coord.x,sph_coord.x FUNC=x-y PERIODIC=NO
abs_y: MATHEVAL ARG=bnz_coord.y,sph_coord.y FUNC=x-y PERIODIC=NO
abs_z: MATHEVAL ARG=bnz_coord.z,sph_coord.z FUNC=x-y PERIODIC=NO
rho: MATHEVAL ARG=abs_x,abs_y,abs_z FUNC=sqrt(x*x+y*y+z*z) PERIODIC=NO
theta: MATHEVAL ARG=abs_z,rho FUNC=acos(x/y) PERIODIC=0.,pi
phi: MATHEVAL ARG=abs_x,abs_y FUNC=atan2(y,x) PERIODIC=-pi,pi

# Restraining potential of the sphere
restr: UPPER_WALLS ARG=rho AT=2.0 KAPPA=1000

# Metadynamics
METAD ...
ARG=rho,theta,phi
GRID_MIN=0,0.,-pi
GRID_MAX=2.2,pi,pi
SIGMA=0.1,pi/16.,pi/8.
HEIGHT=1.2
PACE=500
BIASFACTOR=20
TEMP=300.
LABEL=metad
CALC_RCT
... METAD
```

```
# Printing
PRINT ARG=rho FILE=distance.dat STRIDE=500
PRINT ARG=metad.* FILE=metad_data.dat STRIDE=500
PRINT ARG=restr.* FILE=sphere_restraint.dat STRIDE=500
PRINT ARG=abs_x,abs_y,abs_z FILE=xyz_coord.dat STRIDE=500
PRINT ARG=rho,theta,phi FILE=rtp_coord.dat STRIDE=500
```

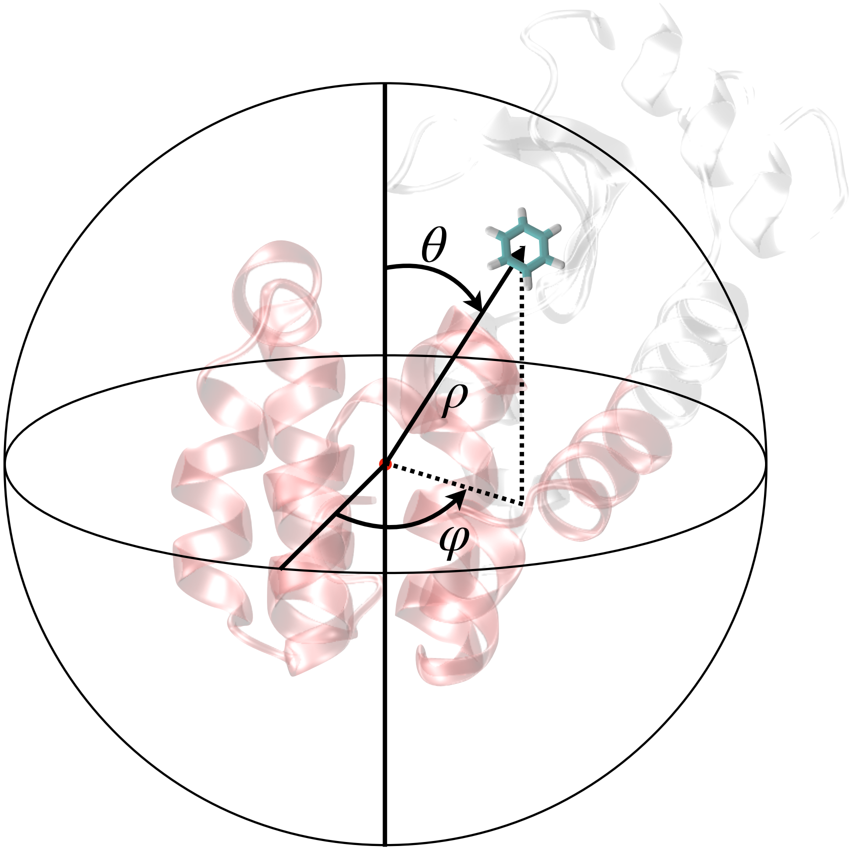


Supplementary Figure 1: Schematic representation of the CVs employed in our metadynamics calculation. The reference frame is fixed on the aligned C-terminal domain of T4L (red, cartoon representation). The spherical coordinates $\rho$, $\theta$, and $\varphi$ that define the position of the benzene (turquoise, licorice representation) are the 3 CVs.

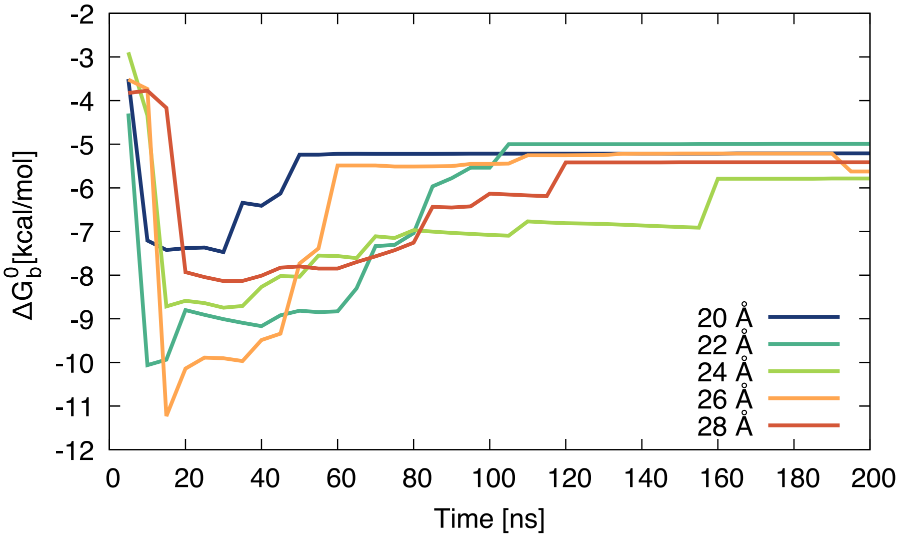


Supplementary Figure 2: Time evolution of the value of $\Delta G_b^0$ for different choices of $\rho_\mathrm{s}$.

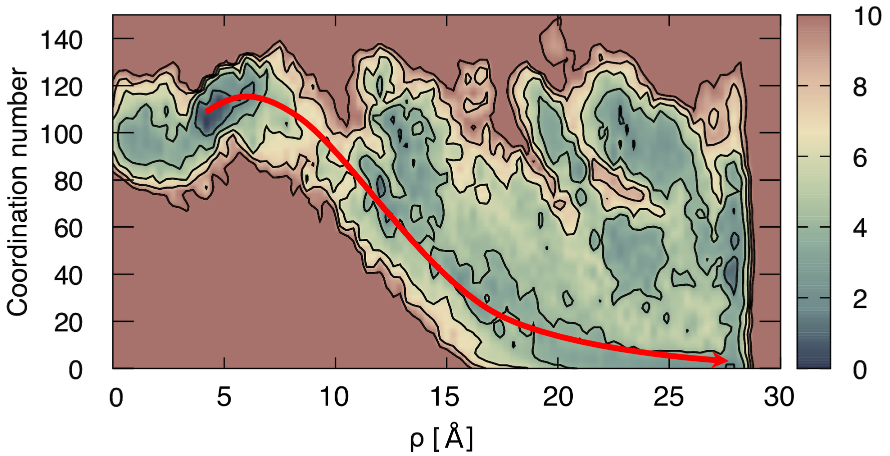


Supplementary Figure 3: Schematic representation of the average of the unbinding pathways. The minimum energy path on the computed FES (here with $\rho_s = 28$ Å) turns out to follow a sigmoidal trend from the bound state to the unbound state, with the inflection point near the radius of gyration of the C-terminal domain, which equal to $\rho_{gyr} = 13.8$ Åin the X-ray structure[2]

.

# References


[1] Finkelstein, A. V.; Janin, J. *Protein Eng., Des. Sel.* **1989**, *3*, 1–3.

[2] Eriksson, A.; Baase, W.; Wozniak, J.; Matthews, B. *Nature* **1992**, *355*, 371.

[3] Maier, J. A.; Martinez, C.; Kasavajhala, K.; Wickstrom, L.; Hauser, K. E.; Simmerling, C. *J. Chem. Theory Comput.* **2015**, *11*, 3696–3713.

[4] Jorgensen, W. L.; Chandrasekhar, J.; Madura, J. D.; Impey, R. W.; Klein, M. L. *J. Chem. Phys.* **1983**, *79*, 926–935.

[5] Wang, J.; Wolf, R. M.; Caldwell, J. W.; Kollman, P. A.; Case, D. A. *J. Comput. Chem.* **2004**, *25*, 1157–1174.

[6] Bayly, C. I.; Cieplak, P.; Cornell, W.; Kollman, P. A. *J. Phys. Chem.* **1993**, *97*, 10269–10280.

[7] Frisch, M. J. et al. Gaussian09. 2009.

[8] Bussi, G.; Donadio, D.; Parrinello, M. *J. Chem. Phys.* **2007**, *126*, 014101.

[9] Parrinello, M.; Rahman, A. *Phys. Rev. Lett.* **1980**, *45*, 1196.

[10] Parrinello, M.; Rahman, A. *J. Appl. Phys. (Melville, NY, U. S.)* **1981**, *52*, 7182–7190.

[11] Essmann, U.; Perera, L.; Berkowitz, M. L.; Darden, T.; Lee, H.; Pedersen, L. G. *J. Chem. Phys.* **1995**, *103*, 8577–8593.
